# Supplementary material for: Transactional Cloud Applications: Status Quo, Challenges, and Opportunities
Source: arXiv:2504.17106 source file (2025-04-23)
Supplement: Supplementary file 1 [file 06_appendix.tex]

\section{Appendix}
\asterios{savepoint here for things that are a bit out of scope. You can copy parts from here, if they fit somewhere in the rest of the paper.}
\subsection{Task Scheduling}

% \rodrigo{Scheduling of tasks and fairness}

In programming languages, an execution model defines how program elements (specified via program syntax) are scheduled for execution~\cite{python_execution}.
Bringing the concept to programming for the cloud, the scheduling of application logic is primarily driven by a combination of the programming model and the underlying systems adopted, in particular the architectural model. In this subsection, we identify three popular alternatives of how application functions are scheduled.

\begin{comment}
\george{
Building applications started with modules tightly coupled to each other in the monolithic approach. The problems of scalability, strong dependencies between different parts of code that should be decoupled, development complexity and many more, pushed the developers for a change, finding an alternative in microservices. Microservices gave the solution with the introduction of independent functionalities communicating via messaging. Although, distinguishing small parts of functionality. Lastly, the introduction of Function as a Service (FaaS) further changed development by enabling versatile and lightweight functions. This style has its own issues to handle, such as autoscaling, messaging guarantees, execution guarantees, and transaction support.
}
\end{comment}

\subsubsection{User-Request Driven}
\label{subsubsec:user_request}
% \textcolor{red}{aka user-request driven task scheduling.}
% In this mode, apart of explicitly provisioning and managing computational resources, users are responsible to specify program concurrency semantics.  

In this model, the network threading model of user-facing components drives task scheduling in the system~\cite{event_loop_nodejs}. 
This is found in the popular three-tier architecture, where application logic execution is driven by client requests. However, it is often the case that there is no order guarantees across clients (e.g., first come first served). Network requests are subject to the underlying operating system packet handling, which may lead some users to experience longer delays~\cite{tailclipper}.

% Furthermore, if the client requests require interacting with the database tier, the DBMS isolation level defined can lead to blocking in case threads contend for data items.

% \noindent\textbf{Decentralized}

% aka choreography. execution like microservices

% Similarly to centralized, application functions can also be triggered by network client requests but they often

Furthermore, a network client request may traverse several components due to the functional partitioning in distributed application architectures ($\S$~\ref{subsub:weak}). Although often leading to a longer end-to-end latency due to increased network I/Os, developers put forth this model to reap benefits associated to high availability. As data is functionally partitioned, the failure of a component usually does not impact the access to data encapsulated by others. The former is achieved as long as the failure does not propagate to other components, which is usually facilitated by the autonomy of components as a design principle. % of event-driven architectures and microservices architectural style. 
 %and  failed components do not affect the execution of others

% However, decentralized execution model introduces challenges not found in centralized mode. Developers are responsible to ensure messaging semantics such as at least once or exactly once delivery. 
%Besides, ACID semantics are usually prohibitive due to distributed commit protocol that introduce many network round trip costs.

% Furthermore, developers need to explicit manage failures and the recovery process of components, a complex task.

\subsubsection{Coordinator/Workers} 
\label{subsubsec:coord_worker}

Apart of the relative simplicity of the user-request model, application developers must handle complex aspects of distributed programming, such as the concurrency semantics of tasks, message delivery semantics, failure handling, resource management, and fairness.
% we are in the cloud, we want to keep some sla, isolation, optimize certain metric, some useful model. allows for more control, optimizing for different metrics.
Furthermore, from a cloud serving model perspective,
the user-request model provides little opportunities to optimize for performance metrics, achieving SLAs, and isolating resources, particularly in multi-component operations.

% Another impedance is that individual components are responsible for system-level concerns, such as failure handling and message processing guarantees.

A traditional model found in high-performance computing that better meets the above requirements is the coordinator/worker pattern~\cite{heron}. In this execution model, 
%instead of client requests driving the execution of the application, 
specific-purpose system components are in charge of scheduling and executing application functions:
%These components are not implemented by developers. 
% uploading application package files (e.g., jar files) or specifying the application functions that are ought to be executed.
a \textbf{\textit{worker}}, whose primary responsibility is receiving and executing tasks; and the \textbf{\textit{coordinator}}, which responsibilities include receiving client requests, dispatching tasks to workers, distributing resources among workers and ensuring fairness. A \textit{worker} is often deployed across a cluster of machines for fault-tolerance and load balancing, and the \textit{coordinator} is often replicated for higher availability, preventing significant service disruptions. Besides its dominance in the stream processing landscape~\cite{heron,flink}, this architectural model is popular in actor systems~\cite{statefun, bykov_orleans_2011} and FaaS architectures~\cite{beldi}.
% distributed stream processing systems like Flink~\cite{flink_arc} (e.g., through \textit{JobManager} and \textit{TaskManagers}) 
% adapted for running stateful functions in the Statefun project~\cite{statefun}.

Depending on the deployment model, the provisioning of computational resources is managed explicitly or offloaded to a cloud provider ($\S$~\ref{subsubsec:resource}).
Independently, it is often the case that application functions are no longer part of an independent deployment unit, like in a monolithic or microservice architecture. % autonomy/sovereignity/independence of application components are lost.
Rather, application functions are either wrapped within the system (i.e., becoming part of the system execution model itself)~\cite{bykov_orleans_2011} or packaged together and submitted to the system, like a \textit{jar} file in Apache Flink~\cite{statefun}, and subject for scheduling across \textit{workers} by the \textit{coordinator}.

% As a result, developers are only responsible for specifying application artifacts that are ought to be executed, such as through \textit{jar} files or application functions (e.g., in the FaaS paradigm).
% Software teams no longer reason about their own deployment units as in the two previous above, but relegate to a system the task of ...
% Although showing slightly differences, this execution model is found in FaaS, dataflows, and actor systems. For instance, in Orleans, coordinator and worker roles intersect in a Silo~\cite{bykov_orleans_2011}. % while in FaaS systems

\subsubsection{Hybrid}

Another recent trend is deploying multiple components (e.g., as microservices) and embedding stateful operators within each to execute data processing tasks. The stateful operators share computational resources with the component.
% run in the same context of the component's deployment unit, sharing computational resources, including the application language runtime memory space (i.e., the heap).
This model originated in the KafkaStreams~\cite{kafka_streams} project and offers an application library for specifying a local dataflow topology. 
Although the components remain independent, the  input and output data of the specified topologies depend on a Kafka~\cite{kafka} broker to operate. For this reason, we characterize it as hybrid execution model, lying between event-driven coordination among components and coordinator/worker (represented by Kafka, with its multiple broker and replica design) models. A particular feature of this model is allowing for operating with application state and streaming state in an unified way.
% https://developer.confluent.io/tutorials/join-a-stream-to-a-table/kstreams.html

\textcolor{red}{perhaps worthy mentioning this could be an interesting option for supporting queryable states?}

% https://www.microsoft.com/en-us/research/uploads/prod/2023/01/unum-nsdi23.pdf
Another emerging pattern in cloud programming is using orchestrators to manage workflows~\cite{dapr_workflow}.
Chaining ($\S$~\ref{subsubsec:function}) and fan-out (i.e., triggering multiple functions) are popular patterns for function composition in the cloud. However, arbitrary compositions, such as through the fan-in pattern,
% ~\cite{dapr_patterns} % some error!?
introduce challenges related to complex control-flow logic and the need to handle crashes, retries, and duplicated messages explicitly~\cite{OrchestratingServerless}. A popular alternative to the above challenges is the use of a so-called "orchestrator." An orchestrator is an independent, long-running, system component that is mainly responsible for ensuring at-least-once or exactly-once delivery guarantees. It sits between an user-request driven ($\S$~\ref{subsubsec:user_request}) and coordinator model ($\S$~\ref{subsubsec:coord_worker}). However, as being a single-point of failure, requires fault-tolerance guarantees and it is shown to limit the performance of workflows in practice~\cite{OrchestratingServerless}.

\subsection{Resource Management}
\label{subsec:resource}

In this subsection, we explore how resource provisioning and isolation, 
such as via containerization, and
lifecycle management, are achieved in the cloud programming landscape.

\subsubsection{Provisioning, Isolation, and Adaptation}
\label{subsubsec:resource}

% \noindent\textbf{Service-oriented Architectures.}
\noindent\textbf{Explicit.} Services are often executed through bare-metal machines or resource virtualization mechanisms, such as virtual machines and containers. Although this scheme allows for isolation in case services share no (logical or physical) resources, as the resources are defined upfront, overprovisioning is a common challenge in service-oriented architectures. This is no different in managed runtimes such as Orleans and Statefun since application maintainers are responsible for provisioning and managing computational resources in a similar manner to services. Besides, actors and stateful functions share computational resources, having developers limited interfaces to configure isolation. Furthermore, resource adaptation is also not transparent in services and managed runtimes. Maintainers must explicitly increase the resources in reaction to higher performance demand, such as increased input rate, an often not optimal measure.
% often not optimal

\noindent\textbf{Transparent.} Serverless runtimes, such as through FaaS systems, obviate the challenges above, offering transparent resource provisioning, function scheduling, failure handling, and elasticity to application maintainers. However, challenges associated to cold starts, execution performance, and costs, undermine a wider adoption of the FaaS paradigm in application architectures \textcolor{red}{(CITE)}.

% Includes fault tolerance, failure handling, scaling, and adapting to dynamic workloads.
% elasticity.
% \textcolor{red}{including resource adaptation}
% Refers to the allocation and management of computational resources for the execution of application functions.
% auto scaling but also preventing few specific components to bottleneck the system or monopolize the computational resources.

\subsubsection{Lifecycle Management}
\label{subsubsec:lifecycle}

The programming abstractions offered to developers ($\S$~\ref{subsec:prog_model}) play a key role in lifecycle management. Managing application objects during runtime, such as actors in the actor model and functions in the FaaS paradigm, is referred to lifecycle management in this subsection.
That includes logical instantiation, localization, failure handling, migration, and free resources used by the application. We categorize lifecycle management into explicit and transparent.

\noindent\textbf{Explicit.} This category appears primarily in service-oriented architectures ($\S$~\ref{subsub:stateless}).   Application maintainers are in charge of deploying services, configuring and detecting failure measures, and implementing recovery procedures. These implicitly includes the objects managed by the application at run time, complexities that only exacerbate the existing challenges of maintaining consistent application states~\ref{subsub:weak}.

% That leads to a burden in ensuring application states remain consistent upon network partitions and failures.

\noindent\textbf{Transparent.} The challenges above motivated the development of distributed systems and frameworks that transparently manage the life cycle of application objects. In frameworks that expose virtual actor abstraction, such as Orleans, users enjoy location and lifecycle transparency. Orleans allocates virtual actors on demand in healthy computational resources and deallocates resources used by actors when they are no longer used. In case of failures, Orleans transparently migrates virtual actors, ensuring that the application remains functional. However, users must handle resource provisioning and scaling explicitly. 
% this is agnostic to deployment technology (container, virtual machine, bare metal). Orleans subsumes node detection failure, node discovery, load balancing, but cannot do horizontal scaling and allocate a new silo. These two must be done explicitly by users, oblivious to the Orleans runtime.

% the computational resources must be provisioned but not explicitly managed by the user, since the Orleans silos coordinate among each other to provide  actor activations (i.e., instantiation) and location transparency, even in the presence of failures.

% https://docs.docker.com/engine/swarm/

% \textbf{Hybrid}
% In other distributed frameworks that exposes virtual actor abstraction, such as Dapr, 
% Virtual actors in Dapr. Within an application, virtual actors' life cycle are managed by Dapr runtime. However, the computational resources must be provisioned and explicitly managed by the user.
% \noindent\textbf{FaaS Systems.}

On the other hand, functions are ephemeral, having a bounded lifecycle (the start and end of a function), managed transparently by a FaaS runtime. Users trigger a function, often through a stateless request over the network, and are oblivious about how or to which computational resource the function will execute. FaaS systems ensure function invocations are scheduled in an individual computational resource, such as a container or a virtual machine~\cite{serverless}. Whenever a function is triggered, its state is brought from storage to the compute node's memory assigned to run the respective function, all transparent to user code.

\subsection{Change Management}
\asterios{take parts of this one, and move to lifecycle management}
\textcolor{red}{observability (aka monitoring), debugging, and data privacy are also very important concerns. maybe observability in resource mgmt and data privacy in state management?}

Change management is a key concern in the software engineering lifecycle and it is no different in cloud applications~\cite{se_cloud,yau2011software}. In a distributed environment, that includes, but not limited to, the deployment, upgrading, and deprecation of components, the updating of the topology and task scheduling strategies, and changes in the data and event schema. The systems and architectures covered in this work play an major role on fulfilling the above.

\noindent\textbf{Service-oriented Architectures.} Data schema changes can be performed without coordinating services when a database per service is used~\cite{Laigner2021}. However, event schema changes require a certain level of coordination among services. The reason is that events trigger functions in downstream components, necessitating matching the producer's and consumers' event schemas.

To alleviate this burden, data serialization systems like Avro~\cite{avro} are used to transparently manage changes in the event schema over time, allowing producers and consumers to remain compatible.
% https://www.ibm.com/topics/avro
However, data serialization tools are oblivious to application state, which can possibly introduce breaking changes. As component tables are often populated using data contained in events~\cite{overeem2021empirical}, populating newly introduced fields is an example of a task that practitioners must treat explicitly~\cite{stack_event_schema}. 
Besides, if application state requires non-null fields, removing fields from the event schema leads to breaking changes.

% api versioning. canary deployment. ad hoc , they build their own tools for that.

% 3.0 to 7.0 Orleans breaking changes
% https://learn.microsoft.com/en-us/dotnet/orleans/migration-guide
On the other hand, service-oriented architectures, by enjoying independence of components, don't forego system-wide breaking changes as in the case of managed services such as Orleans and Statefun. Upgrades can be performed in an isolated manner, not affecting remaining components.

\noindent\textbf{Actor Systems.} Orleans provide grain versioning~\cite{grain_versioning}, a mechanism through which developers can annotate their grain classes indicating an new version. Introducing a new grain version does not require restarting an Orleans cluster. However, rolling out a new grain version require deploying a new silo and deprecating old silos that contain the old grains, a non-trivial task. % ~\cite{grain_version_deploy}. some bug!?
Furthermore, if the new grain version is not backward compatible, calls to the new grain version are always forwarded to a compatible silo, which may limit scalability properties of an Orleans cluster. For last, there is no versioning support to stateless workers and streaming interfaces, impacting changes in scale-out scenarios and streaming workloads, respectively.

% https://github.com/dotnet/orleans/issues/2653

\noindent\textbf{Dataflow Systems.}
Upgrading a dataflow application or migrating it to another cluster often relies on the existence of a consistent snapshot~\cite{upgrade_flink}, obtained via a checkpointing mechanism~\cite{ChandyL85}.
Operators, upon restart, must load their respective states from a snapshot and restart the event processing from the corresponding event stream offset. Besides, as dataflow applications form topologies, changes in the topology also undergo the same process.
% "applications can be upgraded by changing the topology of the application, "
% https://nightlies.apache.org/flink/flink-docs-release-1.20/docs/ops/upgrading/

% One limitation is that
% "Even though Flink consistently restores the state of an application, it cannot revert writes to external systems."
However, upgrading Fink applications is not an automatic process and must be carefully coordinated by application maintainers. Apart of being unable to revert writes to external systems, other challenges with the checkpoint-centric process appear, such as aged snapshots (requiring replaying a lot of events, a long-standing process) and
big state checkpoints (overhead in streaming external storage to operators node).

\subsection{Additional Opportunities}

\subsubsection{Resource Management}

\rodrigo{Execution scheduling. it is an underestimated problem in stateful apps and most of the efforts in this topic are concentrated on serverless functions~\cite{golgi} and container~\cite{res_orc} but unaware of data management tasks at the application/function level}

% cloudburst
% "autoscaling serverless architecture that combines logical disaggregation with physical co-location of compute and storage"
Recent work proposes combining physical co-location of compute and storage by maintaining causally-consistent data in compute node caches~\cite{cloudburst}.

new runtimes and platforms
\cite{skadi,yuanrong}

\subsubsection{Software Engineering Support}

\rodrigo{different aspects. sql. soft eng aspects like OO, how to mainain code, reuse code.
writing whole app in sql. how to test, debug, practical considerations.
complaints about stored proc in these aspects.
virtual actors as a service, like serverless functions.
sql is used in different layers of the system stack today. not a homogeneous. kafka with ksql,ksteeams... 
}

Application development is a costly process (CITE). Being able to forecast challenges related to growing user base, dynamic workloads, system integration, and upgrading the application continuously, through adding modules and schema changes over time, for example, are key concerns when adoption a programming technology for the cloud.

Systems must be designed to allow practitioners to perform SE activities they are able to with traditional software stacks. The lack of debugging, change management, observability, demotivates the use of systems for cloud programming.

\subsubsection{Change Management}

managing event schema changes today is ad hoc. event data and event schema changes must be migrated holistically.

% opportunities. focus is on local changes. clearly missing reasoning about multiple compinents that should "work" together
% https://petereliaskraft.net/res/p2761-li.pdf
% http://www.cs.umd.edu/~abadi/papers/bullfrog-sigmod.pdf

workload fluctuation. new operators, nodes must be made available, these must not jeopardize application responsiveness and up time.

streaming/event rate
